# Supplementary material for: ReCycle: Resilient Training of Large DNNs using Pipeline Adaptation
Source: arXiv:2405.14009 source file (2024-09-25)
Supplement: Supplementary file 1 [file appendix.tex]

\begin{comment}

\appendix
\section{Appendix}
\subsection{Normalization Phase DP Formulation}\label{sec:appendix_dp}


%\noindent\textbf{DP Formulation.}
%Intuitively, the Normalization Phase migrates failures across peer groups and deeper into the pipeline (i.e., to stages with more bubbles).
%To formalize this intuition, we leverage a dynamic programming (DP) solution that determines the ideal location to migrate faults to given a number of failures as shown in Algorithm~\ref{alg:normalization}.

Given the total number of failures to handle, $F$, and the total number of pipeline stages within a data parallel pipeline, $N$, the DP algorithm returns a list $R$ of length $N$, such that $\Sigma_{i} R[i]=F$.
Each index $R[i]$ specifies the ideal number of failures that is assigned to pipeline stage $i$ across all data parallel pipelines; the specific pipeline assignment does not affect performance and can be arbitrary.
For example, if $R[3]=2$ for the example in Figure~\ref{fig:not-recoverable}, the ideal migration would be to swap the failed nodes with any two nodes in stage $3$, for example $W_{0\_3}$ and $W_{2\_3}$.

For each DP step, $C[i][f]$ represents the total cost, in terms of bubbles used, to handle $f$ failures at all stages between $0$ and $i$. 
Meanwhile, each $A[i][f]$ contains a list that denotes the portion of the $f$ failures assigned to each stage from $0$ to $i$, as described for $R$ -- in other words $len(A[i][f]) == i+1$.
Each DP step uses a recurrence relation that aims to minimize the cost of handling $f$ failures within the first $i$ pipeline stages across all of the data parallel pipelines, while $A[i][f]$ denotes the assignment of failures that achieves this cost.
The ideal assignment to handle $F$ failures across all workers is simply $R = A[N-1][F]$.

To estimate the cost, $cost(i, x)$ is a function that returns the extra bubbles used to handle the extra micro-batches from $x$ failures in the $i$-th stage (i.e., peer group).
While we can use the MILP described in Section~\ref{sec:solution} to estimate the cost, the \textit{Planner} can also rely on a heuristic to estimate the cost in order to avoid longer solve times (as Algorithm~\ref{alg:normalization} requires $O(NF)$ calls to the cost function).
The heuristic captures the benefit of the techniques described in Section~\ref{sec:system}.
It creates a pipeline schedule that is similar to 1F1B, except that the heuristic's 1F1B backward pass only schedules $B_{input}$.
Then, when there exists a gap (both in terms of time and memory) that is able to fit $B_{weight}$ (or the $F$ and $B_{input}$ stages are exhausted), $B_{weight}$ operations are scheduled opportunistically.

\subsection{Solution Phase MILP Formulation}\label{sec:appendix_milp}
\noindent\textbf{Notation.}
An operation within a training iteration can be explicitly identified across workers using a 5-tuple $(i, j, k, c, k_s)$.
$i$ represents the pipeline stage within each data parallel pipeline, while $k$ represents the operation's original data parallel pipeline (prior to failures).
$j$ is the micro-batch ID in the training iteration.
$c$ identifies the different operations for each micro-batch, $c \in \{F, B_{input}, B_{weight}\}$.
Finally, $k_s$ denotes the \emph{peer} pipeline in the event that a micro-batch \textit{originally} intended for $k$ runs on $k_s$ (note that $k$ can equal $k_s$).
For example, a micro-batch originally intended to execute on $W_{2\_3}$, but was re-routed to a peer $W_{1\_3}$ in Figure~\ref{fig:recovery-in-recycle}, would have $i=3$, $k=2$, and $k_s=1$.
Thus, $(i, k_s)$ uniquely identifies the worker for a given operation.

\noindent\textbf{Inputs.}
The MILP takes as input the micro-batch to worker assignments in an iteration.
Specifically, the \textit{Planner} takes the normalized failure locations and assigns all micro-batches corresponding to failed workers evenly across peer workers within the same peer group, alongside the original (non-peer) micro-batches.
Thus, the \textit{Planner} produces a binary mapping $S_{i,j,k}^{k_s} \in \{ 0, 1 \}$, which indicates if a micro-batch $(i, j, k)$ should be executed on pipeline $k_s$.
Note that $S_{i,j,k}^{k}=1$ if the micro-batch executes on the original pipeline.
We ensure that each operation is assigned only one pipeline, i.e., \( \sum_{\substack{k_s}} S_{i,j,k}^{k_s} = 1 \).
%Note that $k$ can equal $k_s$.

The MILP also takes as input profiled statistics.
First, $T_c$ represents the computational time for each operation $c$.
$T_{comm}$ represents the communication latency to send activations or gradients across workers\footnote{We use a single value as activations and gradients are the same size.}.
Next, the MILP requires the \textit{change} in memory utilization on worker $(i, k, k_s)$ caused by executing an operation $(i, j, k, c, k_s)$ as \(\Delta M_{i,j,k,c}^{k_s}\).

\begin{equation*}
\Delta M_{i,j,k,c}^{k_s} =
\begin{cases}
    A_{B} & \text{, if } c=F \text{ and  } S_{i,j,k}^{k_s} = 1 \\
    A_B - A_{B_{Input}} & \text{, if } c=B_{Input} \text{ and } S_{i,j,k}^{k_s} = 1 \\
    -A_{B_{Weight}} & \text{, if } c=B_{Weight} \text{ and } S_{i,j,k}^{k_s} = 1 \\
    0 & \text{, otherwise}
\end{cases}
\end{equation*}

Here, \(A_B\) is the profiled size of activation stored at the end of forward pass.
$A_{B_{input}}$ and \(A_{B_{Weight}}\) is size of the activation stored at the end of backward-input and backward-weight pass, respectively.
Upon completion of backward-input pass and backward-weight pass, we free activation \(A_{B_{Input}}\) and \(A_{B_{Weight}}\) respectively.

\noindent\textbf{Variables.}
The goal of the MILP is to identify the exact ordering of operations, which can be used to generate a pipeline schedule.
To do this, we introduce an ordering variable $O_{(i,j,k,c,k_s)\rightarrow(i^\prime,j^\prime,k^\prime,c^\prime,k_s^{\prime})} \in \{ 0, 1 \}$ between each pair of operations $(i, j, k, c, k_s)$ and $(i^\prime, j^\prime,k^\prime,c^\prime,k_s^{\prime})$.
Each variable is 1 if  $(i^\prime, j^\prime,k^\prime,c^\prime,k_s^{\prime})$ is scheduled any time after $(i, j, k, c, k_s)$ and 0 otherwise.
Ordering is only required within a stage, and between computation phases of same micro-batch (e.g., between the $F$ and $B_{input}$ pass).
Finally, we define the set of variables \(E_{i,j,k,c}^{k_s}\) as the ending time of operation \( (i,j,k,c,k_s) \).

\noindent\textbf{Objective.}
The goal of the MILP is to minimize the makespan of a single training iteration (which is repeated throughout the training process).
This can be done by determining the sequence and time of operations through the training pipeline via the sets of variables $O$ and $E$.
This objective can thus be formulated as: 

\begin{equation}
    \min_{\substack{O, E}} \qquad \max_{\substack{i,j,k,k_s}} E_{i,j,k,B_{Weight}}^{k_s} 
\label{eq:ilp-optim-target}
\end{equation}

Here, $\max_{i,j,k,k_s} E_{i,j,k,B_{Weight}}^{k_s}$ represents the end time of the \textit{last} operation in the iteration, representing the makespan.

\noindent\textbf{Constraints.}
The constraints applied to the objective are the following.

\noindent\textit{Cross-Stage Dependencies.}
\begin{equation}
E_{i,j,k,F}^{k_s} \ge 
    S_{i,j,k}^{k_s} \times 
        (\sum_{\hat{k}} (E_{i-1,j,k,F}^{\hat{k}} \times S_{i-1,j,k}^{\hat{k}}) \\ + T_{comm} + T_{F})
\label{eq:ilp-cross-stage-dep-forward}
\end{equation}

% Backward-Input Pass
\begin{equation}
    \begin{multlined}
    E_{i,j,k,B_{Input}}^{k_s} \ge 
        S_{i,j,k}^{k_s} \times
            (\sum_{\hat{k}} (E_{i+1,j,k,B_{Input}}^{\hat{k}} \times S_{i+1,j,k}^{\hat{k}}) \\ + T_{comm} + T_{B_{Input}})
    \end{multlined}
\label{eq:ilp-cross-stage-dep-backward}
\end{equation}

Equation~\ref{eq:ilp-cross-stage-dep-forward} specifies the dependency of a given micro-batch's forward pass on previous pipeline stages (e.g., stage 0 must execute before stage 1).
Similarly, Equation~\ref{eq:ilp-cross-stage-dep-backward} specifies the reverse dependency for the backward pass (e.g., stage 1 must execute before stage 0).

\noindent\textit{Same-Stage Dependencies.}
\begin{equation}
E_{i,j,k,B_{Weight}}^{k_s} \ge 
    S_{i,j,k}^{k_s} \times (E_{i,j,k,B_{Input}}^{k_s} + T_{B_{Weight}})
\label{eq:ilp-same-stage-dep}
\end{equation}

Equation~\ref{eq:ilp-same-stage-dep} allows the MILP to reason about \textit{Decoupled BackProp}, specifying that $B_{input}$ must precede $B_{weight}$ for a given micro-batch within a worker.

\noindent\textit{No Overlapping Computations.}
\begin{equation}
    \begin{multlined}
    E_{i,j^\prime,k^{\prime},c^\prime}^{k_s^{\prime}} \ge 
    E_{i,j,k,c}^{k_s^{\prime}} + T_{c^\prime} - \\ \infty (1 - S_{i,j,k}^{k_s^{\prime}} \times S_{i,j^\prime,k^\prime}^{k_s^{\prime}} + O_{(i,j,k,c,k_s^{\prime})\rightarrow(i,j^\prime,k^\prime,c^\prime,k_s^{\prime})})
    \end{multlined}
\label{eq:ilp-no-overlap}
\end{equation}

Equation~\ref{eq:ilp-no-overlap} adds a dependency constraint which specifies that two different operations cannot overlap in time if they are executed on the same worker.
For example, if operation $(i, j', k', c', k_s^\prime)$ is scheduled after $(i, j, k, c, k_s^\prime)$, they both execute on worker $(i, k_s^\prime)$ and thus $(i, j', k', c', k_s^\prime)$  must begin after $(i, j, k, c, k_s^\prime)$ ends.

\noindent\textit{Memory Constraint.}
\begin{equation}
    \begin{multlined}
    M_{Limit} \ge \Delta M_{i,j^\prime,k^\prime,c^\prime}^{k_s^{\prime}} + \\ \sum_{j,k,c} \Delta M_{i,j,k,c}^{k_s^{\prime}} \times O_{(i,j,k,c,k_s^{\prime})\rightarrow(i,j^\prime,k^\prime,c^\prime,k_s^{\prime})}
    \end{multlined}
\label{eq:ilp-memory}
\end{equation}

Finally Equation~\ref{eq:ilp-memory} calculates the activation memory required at any given time on worker $(i, k_s^\prime)$, and constrains operations such that the total memory is below an $M_{limit}$ to avoid OOMs.
\end{comment}
